# Supplementary material for: GD-GAN: Generative Adversarial Networks for Trajectory Prediction and Group Detection in Crowds
Source: arXiv:1812.07667 source file (2018-12-18)
Supplement: Supplementary file 1 [file 0431-supp.pdf]

# GD-GAN: Generative Adversarial Networks for Trajectory Prediction and Group Detection in Crowds

Tharindu Fernando[1], Simon Denman[1], Sridha Sridharan[1], and Clinton Fookes[1]

Image and Video Research Laboratory, SAIVT, Queensland University of Technology (QUT), Australia.
{t.warnakulasuriya, s.denman, s.sridharan, c.fookes}@qut.edu.au

## 1 Ablation Experiment on the Proposed Trajectory Prediction Model.

To further demonstrate the proposed trajectory prediction approach, we conducted a series of ablation experiments. We utilise the CBE [2] dataset for this experiment and compare the proposed trajectory prediction model against a series of counter parts as follows:

- G / $C_t^h$: We removed the discriminator model and is trained using supervised learning with Mean Square Error (MSE) loss as in [1]. This model only utilises encoded information from the pedestrian of interest, $C_t^s$, defined in Eq. 4 for predicting the future path.
- G: Model G / $C_t^h$ with the the neighbourhood information from Eq. 8. Trained using supervised MSE loss.
- Proposed / $L_1$: We add a discriminator model to G and is trained using the objective defined in Eq. 10. Therefore this model is optimised using the generic GAN objective.

**Table 1.** Ablation experiment results for Proposed trajectory predictor on CBE [2] dataset. Error metrics are as in Sec. 4.2.

| Metric | Dataset | G / $C_t^h$ | G | Proposed /$L_1$ | Proposed |
|---|---|---|---|---|---|
| ADE | Student 003 (CBE) | 1.72 | 0.96 | 0.72 | **0.72** |
| FDE | Student 003 (CBE) | 2.05 | 1.80 | **1.64** | 1.65 |

Considering the ablation experiment results presented in Tab. 1 we observe that model G / $C_t^h$ performs poorly as it generates prediction only considering the trajectory of the pedestrian of interest, without considering the neighbourhood context. We observe an improvement with the addition of $C_t^h$ in model G, still however it fails to outperform the GAN based methods due to the deficiencies with the supervised learning process. With the Proposed /$L_1$ and Proposed models we learn a task specific loss which considers personal and sociological

factors. When comparing Proposed $/L_1$ with Proposed we do not observe any significant performance loss due to the additional sparsity constraint $L_1$ denoting the ability of the proposed method to jointly learn the discriminative group attributes for the group detection task. While the $L_1$ loss does not positively contribute to the trajectory prediction, we note that as shown in the ablation study in Section 4.4 it does lead to improvements in the group detection.

# 2 Using supervised learning for group detection on proposed context features.

**Table 2.** Evaluations of group detection when using supervised learning on proposed context features

| | GD-GAN+ sup | | GD-GAN | |
|---|---|---|---|---|
| | P | R | P | R |
| CEB $\Delta_{GM}$ | **82.7** | **82.3** | 78.7 | 78.7 |
| Student-003 $\Delta_{PW}$ | **83.1** | **74.3** | 80.4 | 68.4 |

Tab. 2 presents the results when using supervised learning approach for group detection on proposed context features.We pass the respective context representation through a SVM classifier which generates the relavant group classification.

## References

1. Fernando, T., Denman, S., Sridharan, S., Fookes, C.: Soft+ hardwired attention: An lstm framework for human trajectory prediction and abnormal event detection. arXiv preprint arXiv:1702.05552 (2017)
2. Lerner, A., Chrysanthou, Y., Lischinski, D.: Crowds by example. In: Computer Graphics Forum. vol. 26, pp. 655–664. Wiley Online Library (2007)
